# Supplementary material for: Emergent Bistability and Switching in a Nonequilibrium Crystal
Source: arXiv:1706.04311 ancillary file (2017-09-25)
Supplement: Supplementary file 1 [file supplemental.pdf]

# Supplemental Information — Emergent Bistability and Switching in a Nonequilibrium Crystal

Guram Gogia and Justin C. Burton

*Department of Physics, Emory University, Atlanta, GA, 30322*

**Supplementary Video 1.** Bistable switching. Three cycles of melting and re-crystallization for 314 particles with mean diameter = 9.46 $\mu$m at P = 1.05 Pa and $V_{bias}$ = -7.6 V. The diameter of the sample is 3.6 cm. The slow rotation of the sample is due to the vertical component of Earth's magnetic field [1].

**Supplementary Video 2.** Bistable Switching. Three cycles of melting and re-crystallization for 1532 particles with mean diameter = 8 $\mu$m at P = 0.92 Pa and $V_{bias}$ = -17.6 V. The diameter of the sample is 5.2 cm. The slow rotation of the sample is due to the vertical component of Earth's magnetic field [1].

**Supplementary Video 3.** Bistable Switching. One cycle of melting and re-crystallization for 691 particles with mean diameter = 9.46 $\mu$m at P = 0.79 Pa and $V_{bias}$ = -7.4 V. The width of the shown section is 2.6 cm.

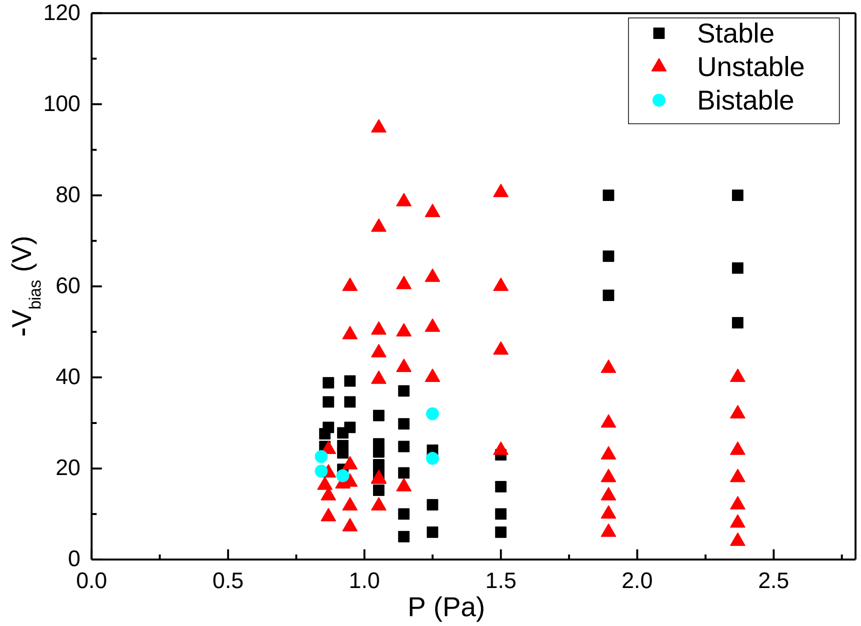


FIG. S1. Phase diagram of a system consisting of 1443 melamine-formaldehyde particles with diameter of 8 $\mu$m.

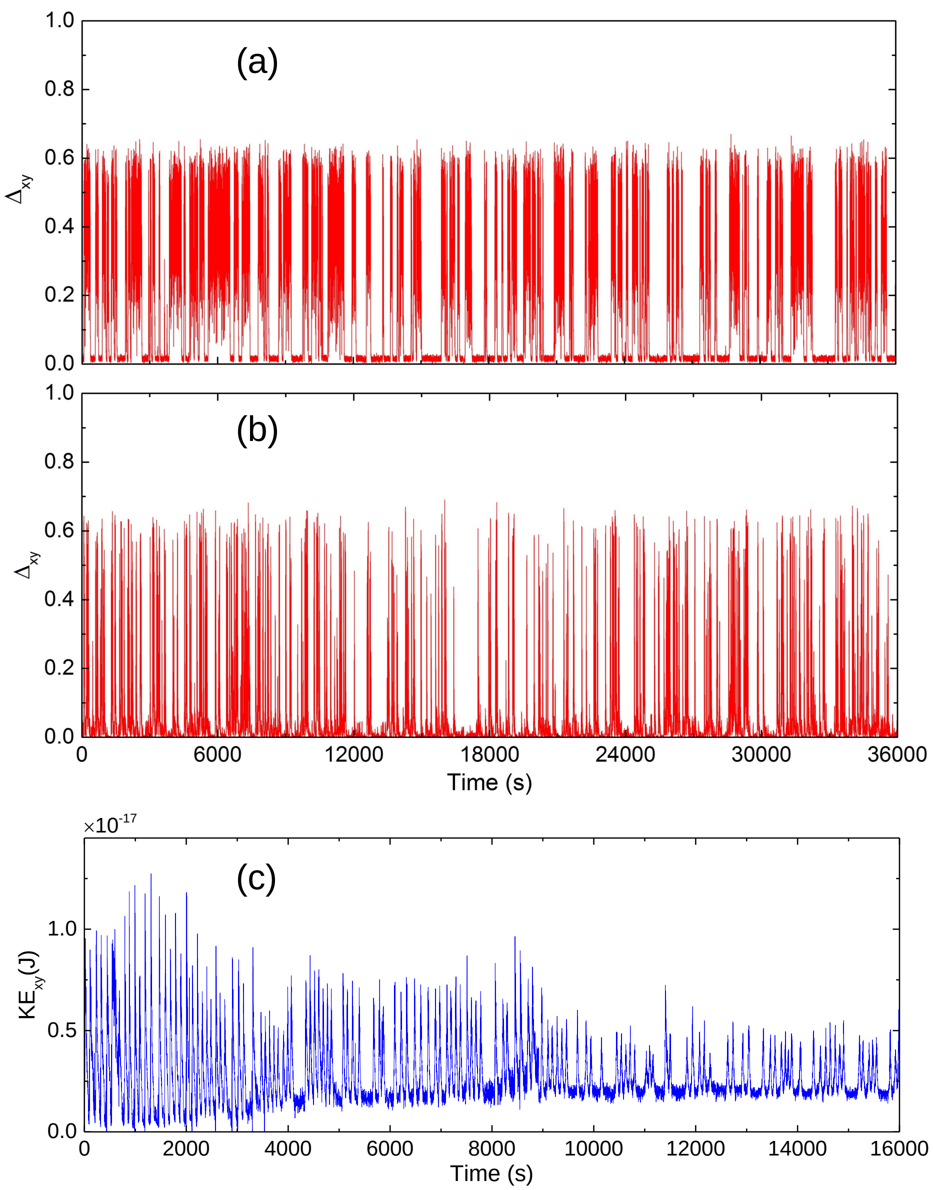


FIG. S2. Switching dynamics of both the simulation and experiment over long times. (a)-(b) Simulation results showing the evolution of $\Delta_{xy}$ for (a) 500 particles and (b) 1000 particles. (c) Horizontal kinetic energy $KE_{xy}$ in our experiments for 723 particles with a mean diameter of 9.46 $\mu$m. The gas pressure was $P$ = 0.73 Pa and $V_{bias}$ = -2.88 V. The peaks of $KE_{xy}$ become less and less pronounced as the time goes on because the particles lose mass due to plasma interactions [2], and consequently the monolayer destabilizes. The parameters for the simulations are described in the main text.

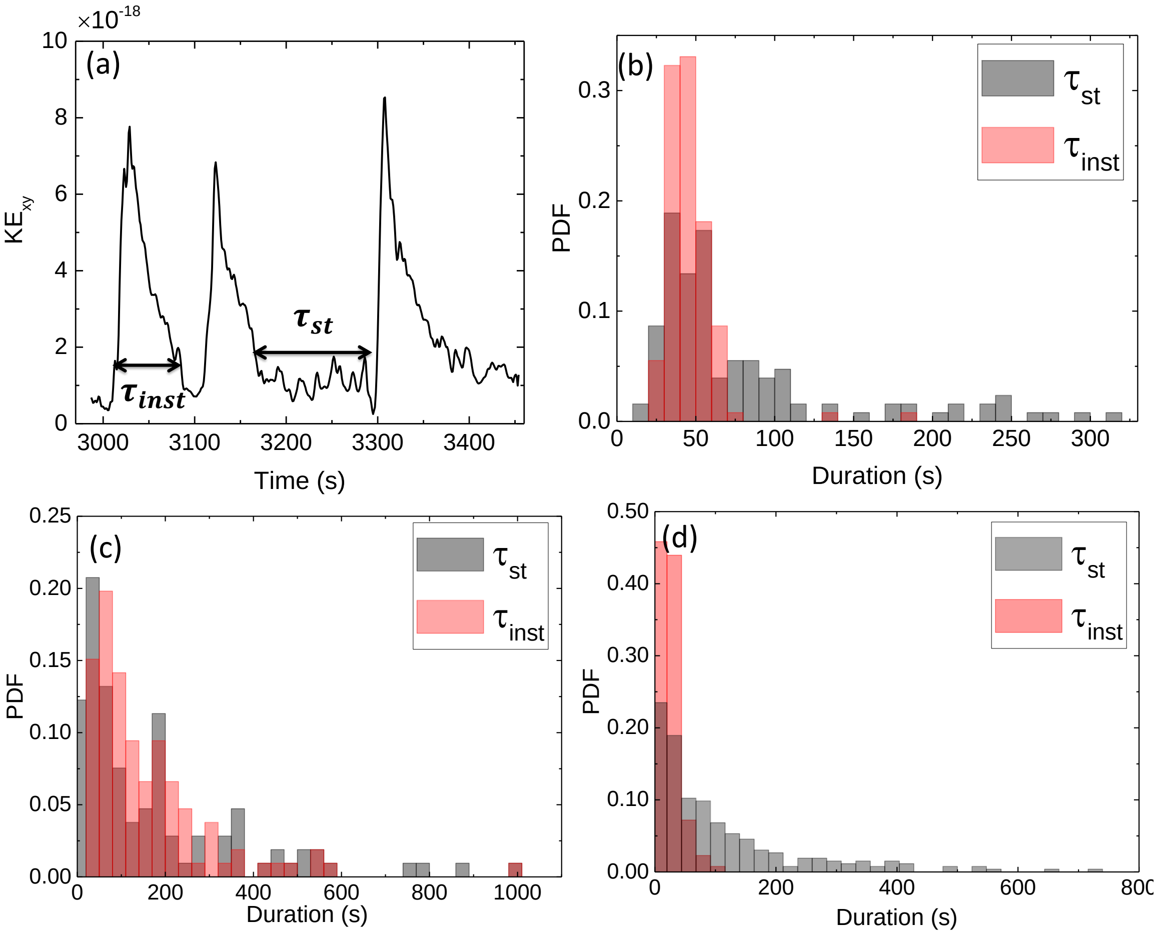


FIG. S3. Distributions of stability (crystalline) and instability (gas-like) periods in the experiment and simulations. (a) The durations of two distinct phases are defined by thresholding the horizontal kinetic energy at $KE_{xy} = 2.0 \times 10^{-18}$ J. Below the threshold the system is in stable phase, whereas above the threshold the system is unstable. (b) The distributions of $\tau_{st}$ and $\tau_{inst}$ in the experiment for for 723 particles with a mean diameter of 9.46 $\mu$m. The gas pressure was $P = 0.73$ Pa and $V_{bias}$ = -2.88 V. For comparison, distributions are also shown for simulations of 500 and 1000 particles in (c) and (d), respectively. The parameters for the simulations are described in the main text.

[1] U. Konopka, D. Samsonov, A. V. Ivlev, J. Goree, V. Steinberg, and G. E. Morfill, Phys. Rev. E **61**, 1890 (2000).

[2] J. Pavlu, A. Velyhan, I. Richterova, Z. Nemecek, J. Safrankova, I. Cermak, and P. Zilavy, IEEE Trans. Plasma Sci. **32**, 704 (2004).
